# Supplementary material for: Conditional Imitation Learning for Multi-Agent Games
Source: arXiv:2201.01448 source file (2022-01-05)
Supplement: Supplementary file 1 [file split_appendix.tex]

\documentclass{article}

\usepackage{pdfpages}

\usepackage{bashful}

\begin{document}

\bash
latexmk -pdf main >& /dev/null
\END

\includepdf[pages=12-]{main}

\end{document}
